# Supplementary material for: Unphysical Discontinuities, Intruder States and Regularization in $GW$ Methods
Source: arXiv:2202.11589 source file (2022-05-01)
Supplement: Supplementary file 1 [file ufGW-SI.pdf]

# Supplementary Material for "Unphysical Discontinuities, Intruder States and Regularization in $GW$ Methods"


Enzo Monino[1] and Pierre-François Loos[1, a)]

*Laboratoire de Chimie et Physique Quantiques (UMR 5626), Université de Toulouse, CNRS, UPS, France*


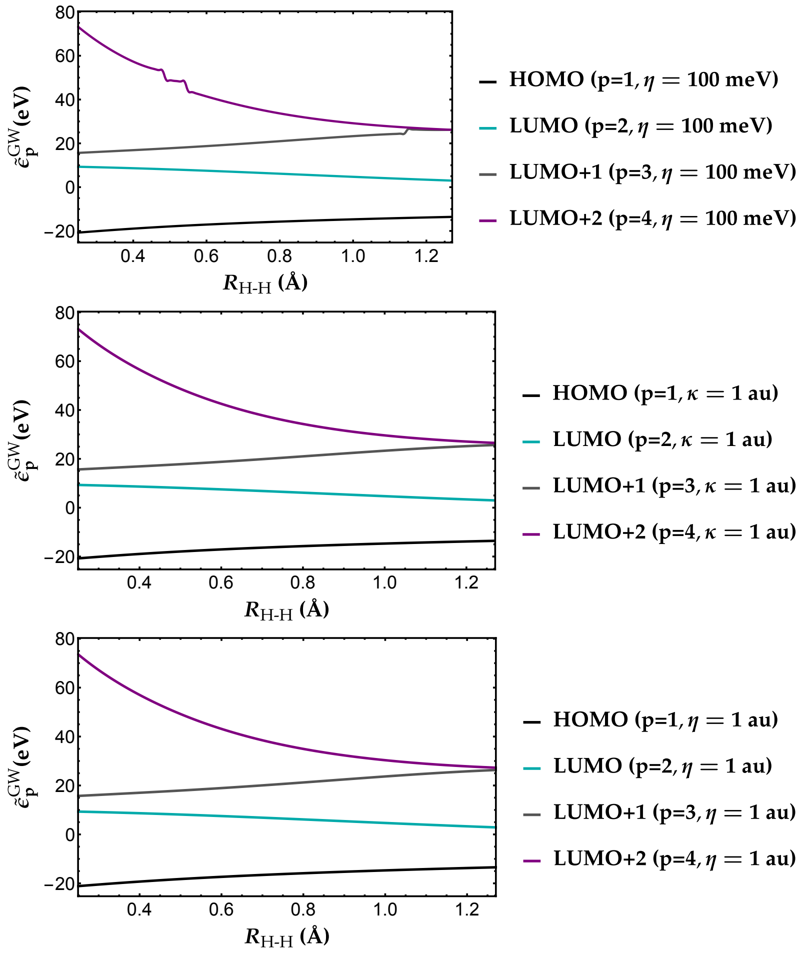


FIG. 1. Regularized quasiparticle energies $\tilde{\epsilon}_p^{GW}$ as functions of the internuclear distance $R_{\text{H–H}}$ (in Å) of $H_2$ at the $G_0W_0$@HF/6-31G level for $\eta = 100$ meV (top), $\eta = 1\,E_\text{h}$ (center), and $\kappa = 1\,E_\text{h}$ (bottom).


a)Electronic mail: loos@irsamc.ups-tlse.fr

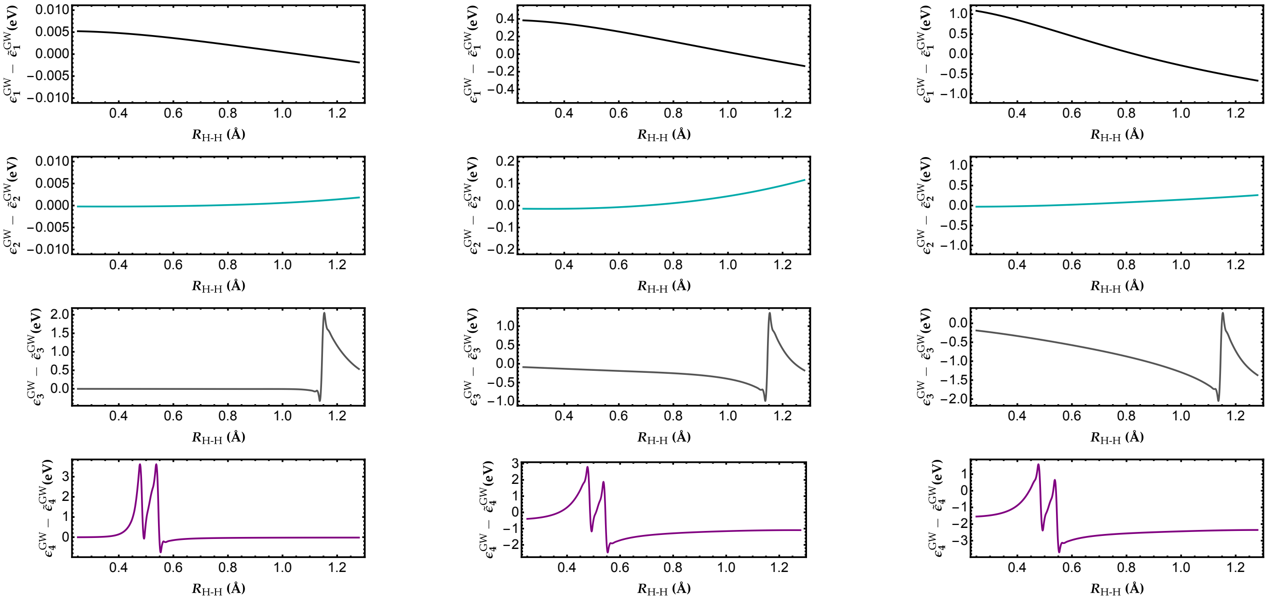


FIG. 2. Difference between non-regularized and regularized quasiparticle energies $\epsilon_p^{GW} - \tilde{\epsilon}_p^{GW}$ computed with $\eta = 0.1\,E_\text{h}$ (left), $\eta = 1\,E_\text{h}$ (center), and $\eta = 10\,E_\text{h}$ (right) as functions of the internuclear distance $R_{\text{H-H}}$ (in Å) of $H_2$ at the $G_0W_0$@HF/6-31G level.

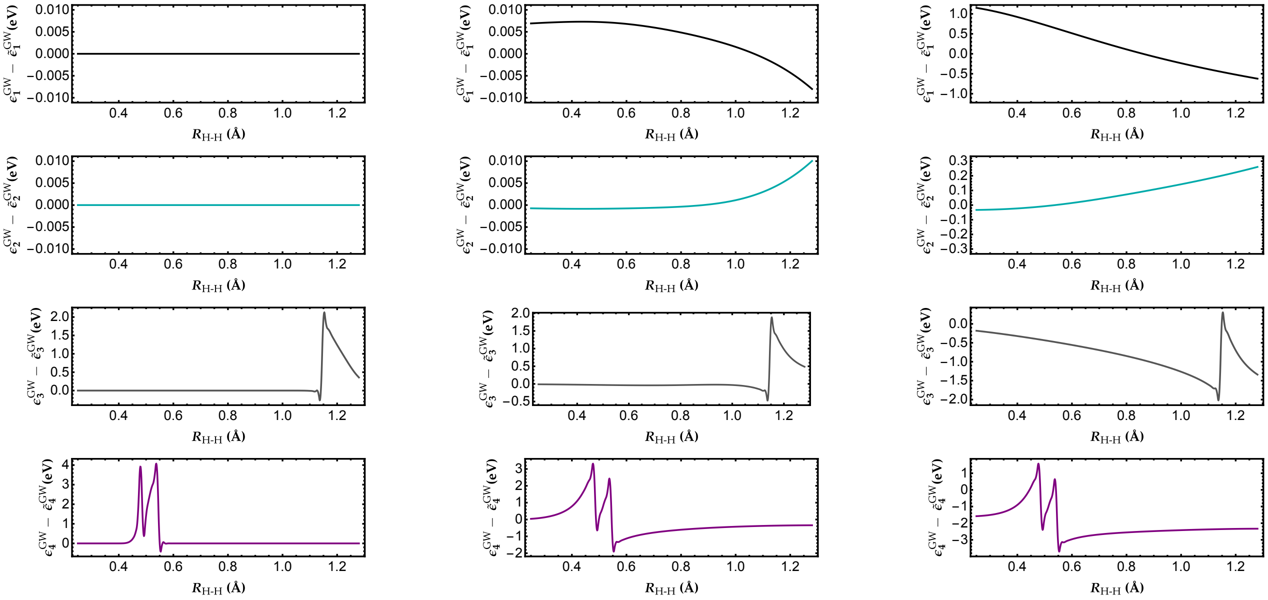


FIG. 3. Difference between non-regularized and regularized quasiparticle energies $\epsilon_p^{GW} - \tilde{\epsilon}_p^{GW}$ computed with computed with $\kappa = 0.1\,E_\text{h}$ (left), $\kappa = 1\,E_\text{h}$ (center), and $\kappa = 10\,E_\text{h}$ (right) as functions of the internuclear distance $R_{\text{H-H}}$ (in Å) of $H_2$ at the $G_0W_0$@HF/6-31G level.

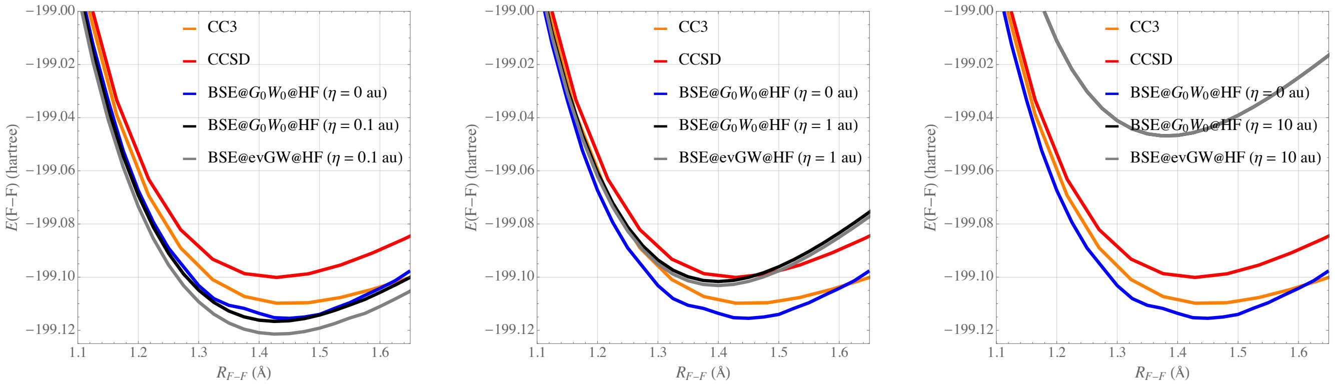


FIG. 4. Ground-state potential energy surface of $F_2$ around its equilibrium geometry obtained at various levels of theory with the cc-pVDZ basis set for $\kappa = 0.1\,E_\text{h}$ (left), $\eta = 1\,E_\text{h}$ (center), and $\eta = 10\,E_\text{h}$ (right).

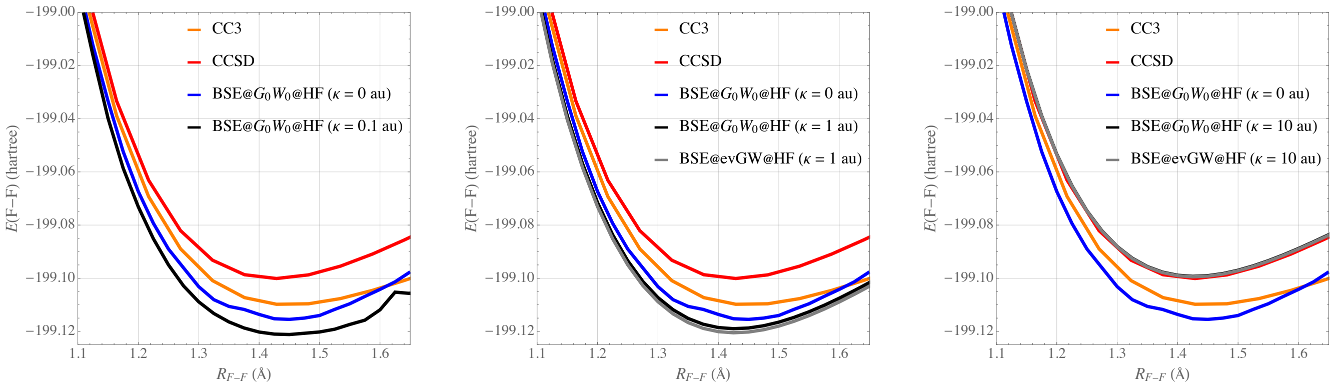


FIG. 5. Ground-state potential energy surface of $F_2$ around its equilibrium geometry obtained at various levels of theory with the cc-pVDZ basis set for $\kappa = 0.1\,E_\text{h}$ (left), $\kappa = 1\,E_\text{h}$ (center), and $\kappa = 10\,E_\text{h}$ (right). For $\kappa = 0.1\,E_\text{h}$, the BSE@ev$GW$@HF calculations do not converge for numerous values of $R_{\text{F−F}}$ and are not shown in this figure. For $\kappa = 10\,E_\text{h}$, the black and gray curves are superposed.
